# Supplementary material for: Renaissance of Literate Programming in the Era of LLMs: Enhancing LLM-Based Code Generation in Large-Scale Projects
Source: arXiv:2502.17441 source file (2024-12-25)
Supplement: Supplementary file 1 [file mini-goldfish.tex]

\section{Mini-goldfish document}

To test the model's ability to focus on a document, we provided a smaller new document named Mini-goldfish. In the document, we provide details of three cases of writing programs in the Functional Programming pattern. It is exactly write a Chain of Thought template in a document. We also list the defined procedures in a chapter named Index.

To specify the generating of codes, we write the document in a recursive pattern, which is named as the Skeleton of a chunk. For example,

\begin{figure*}[ht]
  \centering
  \includegraphics[width=0.8\textwidth]{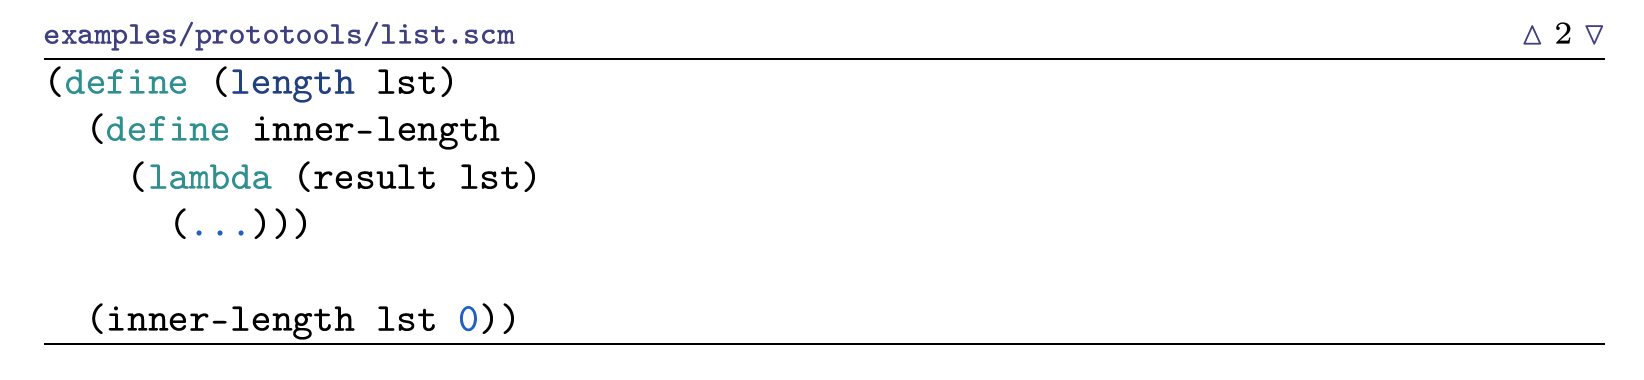}
  \caption{Write your code in an inner recursive pattern}
  \label{fig:inner-rec}
\end{figure*}

The chunk in Fig.\ref{fig:inner-rec} defines a procedure to get the length of a list. The implementation is based on a recursive way, which defines an inner procedure named "inner-length," which receives two parameters. As a result, the procedure "length" we need is just an instance of the inner procedure with an accumulator, the number $0$. This design provides an easy way to check whether the models have learned our FP pattern well.

\section{Testing LLMs with Mini-goldfish and Goldfish Scheme}

% \begin{figure*}[ht]
%    \centering
%       \includegraphics[width=\textwidth]{figures/curr_outline_2.png}
%       \caption{Current outlines of selling points}
%    \label{fig:inner-rec}
% \end{figure*}

To evaluate LLMs' ability to focus on specific documentation, we developed Mini-goldfish based on the  Goldfish Scheme LP document \yl{why should we use mini-goldfish instead of goldfish itself?}. The mini-goldfish document serves as a controlled \yl{what do you mean by controlled? control what?} test environment for assessing LLMs' code generation capabilities within the context of Goldfish Scheme.

\subsection{The Mini-goldfish Document Structure}

Mini-goldfish contains three essential components \yl{why should the reviewer care about these structures? mention the challenge before you introduce the design method. Then, discuss why the design works.}:
\begin{enumerate}
  \item Examples demonstrating Functional Programming (FP) patterns % If FP is defined, then remove the thing out of ()
  \item Chain of Thought documentation explaining implementation reasoning
  \item An Index chapter listing all available procedures
\end{enumerate}

This structured approach enables precise tracking of whether LLMs utilize only the provided tools and patterns. The document effectively creates a controlled environment for testing code generation capabilities.
